# Supplementary material for: PRISM: Periodic Representation with multIscale and Similarity graph Modelling for enhanced crystal structure property prediction
Source: arXiv:2511.20362 source file (2025-11-25)
Supplement: Supplementary file 1 [file PRISM_SI.pdf]

# Supplementary Information

Àlex Solé,<sup>†,‡</sup> Albert Mosella-Montoro,<sup>†</sup> Joan Cardona,<sup>‡</sup> Daniel Aravena,<sup>\*,¶</sup> Silvia Gómez-Coca,<sup>\*,‡</sup> Eliseo Ruiz,<sup>\*,‡</sup> and Javier Ruiz-Hidalgo<sup>\*,†</sup>

<sup>†</sup>*Image Processing Group - Signal Theory and Communications Department, Universitat Politècnica de Catalunya, Barcelona, Spain*

<sup>‡</sup>*Inorganic and Organic Chemistry Department and Institute of Theoretical and Computational Chemistry, Universitat de Barcelona, Barcelona, Spain*

<sup>¶</sup>*Materials Chemistry Department, Faculty of Chemistry and Biology, Universidad de Santiago de Chile, Santiago, Chile*

E-mail: daniel.aravena.p@usach.com; silvia.gomez@qi.ub.es; eliseo.ruiz@qi.ub.edu; j.ruiz@upc.edu

## Detailed Architecture

This section outlines the necessary adaptations to convert a baseline architecture into the proposed PRISM pipeline. Starting from existing pipelines designed for crystal structures, such as iComformer,<sup>1</sup> eComformer,<sup>1</sup> or CartNet,<sup>2</sup> the initial atom and edge encoders remain unchanged. The primary modification involves the integration of a Superatom Encoder and minimal alterations to the message-passing mechanism to accommodate the Multiscale Expert, which lacks explicit geometric edge information. The subsequent subsections provide comprehensive details on the Superatom Encoder implementation and outline the specific adjustments made to CartNet, enabling the construction of the complete PRISM architecture. Although this description focuses on CartNet, the proposed changes can be adapted similarly to any other baseline architecture, as demonstrated in the Discussion Section of the main

## Superautom Encoder

This module creates the initial embedding representation of the supernode  $s$ , which is in charge of the more global representations of the crystal and encodes the repetitions of the crystal structure via Cell Expert.

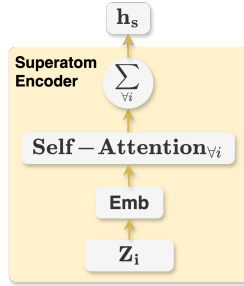

Figure 1: Schematic of the Superautom encoder. It performs self-attention between all the nodes in  $\mathcal{V}$  and aggregates all of them in a single representation.

Figure 1 shows a schematic of the Superautom encoder. Initially, each atom  $i$  in the unit cell  $\mathcal{V}$  is assigned an embedding  $\mathbf{z}_{\text{cell},i}$  based on its atomic number. Subsequently, each atom embedding is updated via a self-attention mechanism considering all other atoms within the unit cell as follows:

$$\alpha_{ij} = \frac{e^{\frac{\mathbf{q}_i^T \mathbf{k}_j}{\sqrt{\dim}}}}{\sum_{\forall u \in \mathcal{V}} e^{\frac{\mathbf{q}_i^T \mathbf{k}_u}{\sqrt{\dim}}}} \quad (1)$$

$$\mathbf{f}_i = \sum_{\forall j \in \mathcal{V}} \alpha_{ij} \mathbf{v}_j, \quad (2)$$

where  $\mathbf{q}_i$ ,  $\mathbf{k}_j$ , and  $\mathbf{v}_j$  represent learnable linear projections of the initial atomic embeddings  $\mathbf{z}_{\text{cell}}$ , and  $\alpha_{ij}$  is the Softmax function of  $\mathbf{q}_i^T \mathbf{k}_j / \sqrt{\dim}$ . Finally, the embeddings  $\mathbf{f}_i$  from all atoms are summed to form the initial embedding for the supernode  $s$ , denoted as  $\mathbf{h}_s^{(0)}$ :

$$\mathbf{h}_s^{(0)} = \sum_{\forall i \in \mathcal{V}} \mathbf{f}_i. \quad (3)$$

## Baseline Modification

This section details the modifications necessary for adapting a baseline architecture into the PRISM pipeline. While the following description specifically addresses the adjustments required for CartNet,<sup>2</sup> due to its results highlighted in the Discussion Section from the main manuscript, these modifications can be generalised and have been applied to other baseline architectures designed for crystal structures. Figure 2 illustrates the modules employed within the CartNet baseline. Atom nodes and edges are initialised using consistent Atom and Edge Encoders, respectively, and the CartLayer serves as the primary message-passing module utilised by our aggregation experts.

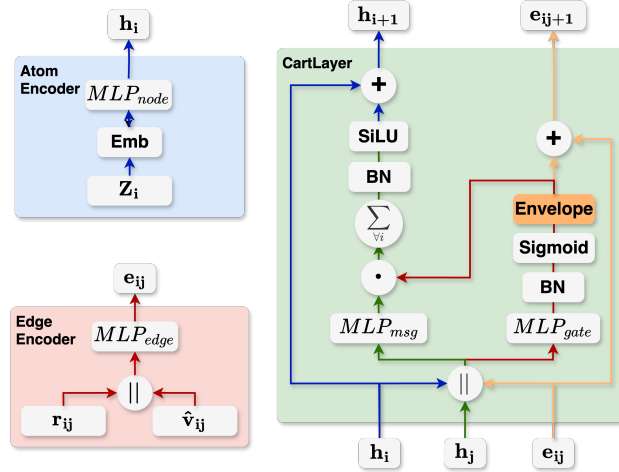

Figure 2: Schematic of our detailed blocks used in CartNet. The Atom Encoder (blue) maps discrete atomic features into continuous embeddings via a MLP. The Edge Encoder (red) computes interatomic distances and directions, encodes distances with a set of Radial Basis Functions (RBF), and processes them through a MLP. The CartLayer (green) performs gated message passing with an explicit Envelope function. Orange paths indicate branches omitted in the Multiscale Expert variant.

## Atom Encoder

This module encodes the initial atomic representations  $h_i$  and it has no modifications from the original design. Each atom  $i$  has its own atomic number  $z_i$ . We map  $z_i$  into  $\mathbb{R}^{dim}$  via an embedding  $\text{Emb}(z_i)$ , and then apply a small MLP to obtain the initial hidden node feature  $\mathbf{h}_i \in \mathbb{R}^{dim}$ :

$$\mathbf{h}_i = \text{MLP}_{\text{node}}(\text{Emb}(z_i)). \quad (4)$$

The  $\text{MLP}_{\text{node}}$  consists of two linear layers: the first layer doubles the embedding dimension, applies a SiLU activation; the second layer projects back to  $dim$  and applies another SiLU. This yields a smoothly non-linear mapping from the raw embedding into the hidden space.

## Edge Encoder

The Edge Encoder is responsible for encoding the necessary geometrical information needed for the edges. In our PRISM baseline, the Edge Encoder is used three times, the first one to encode the edges for the atomistic neighbourhood, the second to encode the cell edges in the cell neighbourhood and finally for the feature-space neighbourhood which is used per layer.

An edge  $(i, j)$  connects receiver atom  $i$  and sender atom  $j$ . From their positions  $\mathbf{r}_i, \mathbf{r}_j \in \mathbb{R}^3$  we compute:

$$d_{ij} = \|\mathbf{r}_j - \mathbf{r}_i\|, \quad (5)$$

$$\hat{\mathbf{v}}_{ij} = (\mathbf{r}_j - \mathbf{r}_i)/d_{ij}. \quad (6)$$

We then encode the scalar distance  $d_{ij}$  into a  $K$ -dimensional radial-basis (RBF) vector  $\boldsymbol{\rho}_{ij}$  via

$$\rho_k(d_{ij}) = \exp(-\beta(\exp(-d_{ij}) - \mu_k)^2), \quad k = 0, \dots, K-1, \quad (7)$$

with fixed centers  $\mu_k$  and width  $\beta$ .  $\mu$  is initialized with equally spaced values between  $\exp(-r_c)$  and 1, and  $\beta$  are initialized with a fixed  $\beta = (2K^{-1}(1 - \exp(-r_c)))^{-2}$

Concatenating  $\boldsymbol{\rho}_{ij}$  with  $\hat{\mathbf{v}}_{ij}$ , we obtain the edge feature

$$\mathbf{e}_{ij} = \text{MLP}_{\text{edge}}([\boldsymbol{\rho}_{ij} \parallel \hat{\mathbf{v}}_{ij}]). \quad (8)$$

Here  $\text{MLP}_{\text{edge}}$  also has two linear layers: the first doubles the input dimension  $dim$  and applies SiLU, the second returns to  $dim$  and applies SiLU.

In our specific PRISM scenario, for the atomistic and feature-space neighbourhood, RBF is initialised with  $r_c$ , and for the cell neighbourhood is initialised using  $R_c$ , where  $R_c \gg r_c$ . For the feature-space neighbourhood, before the computation of the of the distance  $d_{ij}$  and the direction vector  $\hat{\mathbf{v}}_{ij}$ , the minimal distance between repetitions is found using the equations described in the Methodology Section from the main manuscript.

### Message-Passing Module

The Message-Passing Module is in charge to share information between nodes and/or supernodes. In our specific pipeline, the Message-Passing Module is used 4 times, one for each expert (Cell, Multiscale, Atomistic, and Similarity).

At each module, sender and receiver node features  $\mathbf{h}_i, \mathbf{h}_j$  and edge feature  $\mathbf{e}_{ij}$  are combined into a gate and a message. The gate is:

$$\mathbf{g}_{ij} = \sigma(\text{BN}(\text{MLP}_{\text{gate}}[\mathbf{h}_i \parallel \mathbf{e}_{ij} \parallel \mathbf{h}_j])) \odot \text{Env}(d_{ij}), \quad (9)$$

where  $\text{MLP}_{\text{gate}}$  first projects the  $3dim$  input down to  $dim$ , applies SiLU, then projects within  $dim$  again; its output is batch-normalized and passed through a sigmoid.

The Envelope function is defined as:

$$\text{Env}(d_{ij}) = \frac{1}{2} \left( \cos\left(\frac{\pi d_{ij}}{r_c}\right) + 1 \right), \quad (10)$$

which smoothly decays interactions near the cutoff  $r_c$ .

In parallel, the raw message is:

$$\tilde{\mathbf{m}}_{ij} = \text{MLP}_{\text{msg}}[\mathbf{h}_i \parallel \mathbf{e}_{ij} \parallel \mathbf{h}_j], \quad (11)$$

where  $\text{MLP}_{\text{msg}}$  first projects the  $3dim$  input down to  $dim$ , applies SiLU, then projects within  $dim$  again; but without batch-norm or sigmoid. We then weight it by the gate:

$$\mathbf{m}_{ij} = \tilde{\mathbf{m}}_{ij} \odot \mathbf{g}_{ij}. \quad (12)$$

Aggregating over neighbours  $\mathcal{N}_i$  and applying batch-norm + SiLU with a residual connection yields:

$$\mathbf{h}'_i = \mathbf{h}_i + \text{SiLU}\left(\text{BN}\left(\sum_{j \in \mathcal{N}_i} \mathbf{m}_{ij}\right)\right), \quad (13)$$

$$\mathbf{e}'_{ij} = \mathbf{e}_{ij} + \mathbf{g}_{ij}. \quad (14)$$

For the multiscale expert (orange paths in Figure 2), we omit the edge encoder and gating branches: messages are computed solely from the concatenated node embeddings and aggregated without updating any  $\mathbf{e}_{ij}$ .

## Head

The final atomic embeddings  $\mathbf{h}_i^{\text{final}} \in \mathbb{R}^{dim}$  are processed through a multilayer perceptron (MLP) to produce individual atomic predictions. Specifically, the MLP consists of two linear layers with weights  $\mathbf{W}_1 \in \mathbb{R}^{\frac{dim}{2} \times dim}$ ,  $\mathbf{W}_2 \in \mathbb{R}^{1 \times \frac{dim}{2}}$  and biases  $\mathbf{b}_1 \in \mathbb{R}^{\frac{dim}{2}}$ ,  $\mathbf{b}_2 \in \mathbb{R}^1$ , separated by a SiLU activation function:<sup>3</sup>

$$o_i = \mathbf{W}_2 \text{SiLU}(\mathbf{W}_1 \mathbf{h}_i^{\text{final}} + \mathbf{b}_1) + \mathbf{b}_2, \quad (15)$$

where the SiLU activation function is used as non-linearity.

The final property prediction  $y$  for the crystal is obtained by averaging these atomic-level

predictions, thus capturing comprehensive local-to-global structural and chemical contexts while naturally preserving the physical symmetries inherent in crystalline materials:

$$y = \frac{1}{N} \sum_{i=1}^N o_i. \quad (16)$$

Where  $N$  is the number of atoms in the unit cell  $\mathcal{V}$ .

## Scalability and Computational Cost

In our PRISM framework, each graph edge corresponds to a single message passed during inference, and thus the total number of edges, equivalently, the total number of messages, governs the computational cost. We decompose the total edge count, denoted  $\mathcal{E}_{\text{total}}$ , into four disjoint components:

$$\mathcal{E}_{\text{total}} = \mathcal{E}_{\text{atomistic}} + \mathcal{E}_{\text{cell}} + \mathcal{E}_{\text{feat}} + \mathcal{E}_{\text{multiscale}} \quad (17)$$

The multiscale expert connects each of the  $N$  atomic nodes from the unit cell  $\mathcal{V}$  bidirectionally to a global superatom, yielding

$$\mathcal{E}_{\text{multiscale}} = 2N \quad (18)$$

Showing a linear relation between the computational cost and the number of atoms  $N$ .

By contrast, the atomistic and cell edges depend on the neighbour counts within fixed cutoff radii and must be estimated empirically. The feature-space expert produces edges according to learned similarity thresholds, which depend on the model, training data, and optimization, which implies that also must be estimated empirically. Figure 3 illustrates the scaling behavior of each edge component on a log-log axis. For small unit cells ( $N \lesssim 10$ ),  $\mathcal{E}_{\text{cell}}/N$  is relatively large: compact lattice vectors place many periodic images within the cell-space cutoff, producing dense superatom connectivity. In contrast,  $\mathcal{E}_{\text{atomistic}}/N$ ,  $\mathcal{E}_{\text{multiscale}}/N$ , and  $\mathcal{E}_{\text{feat}}/N$  remain low, since few geometric neighbours fall inside the atomistic radius, the

multiscale edges contribute exactly two per atom, and feature-space edges are limited by learned similarity thresholds. As the number of atoms grows, the lattice expands (reducing  $\mathcal{E}_{\text{cell}}/N$ ) while more Euclidean neighbours lie within the atomistic cutoff, increasing  $\mathcal{E}_{\text{atomistic}}/N$ ; the multiscale term grows linearly and feature edges remain a small, roughly constant fraction (see the lower-left and lower-right panels of Figure 3).

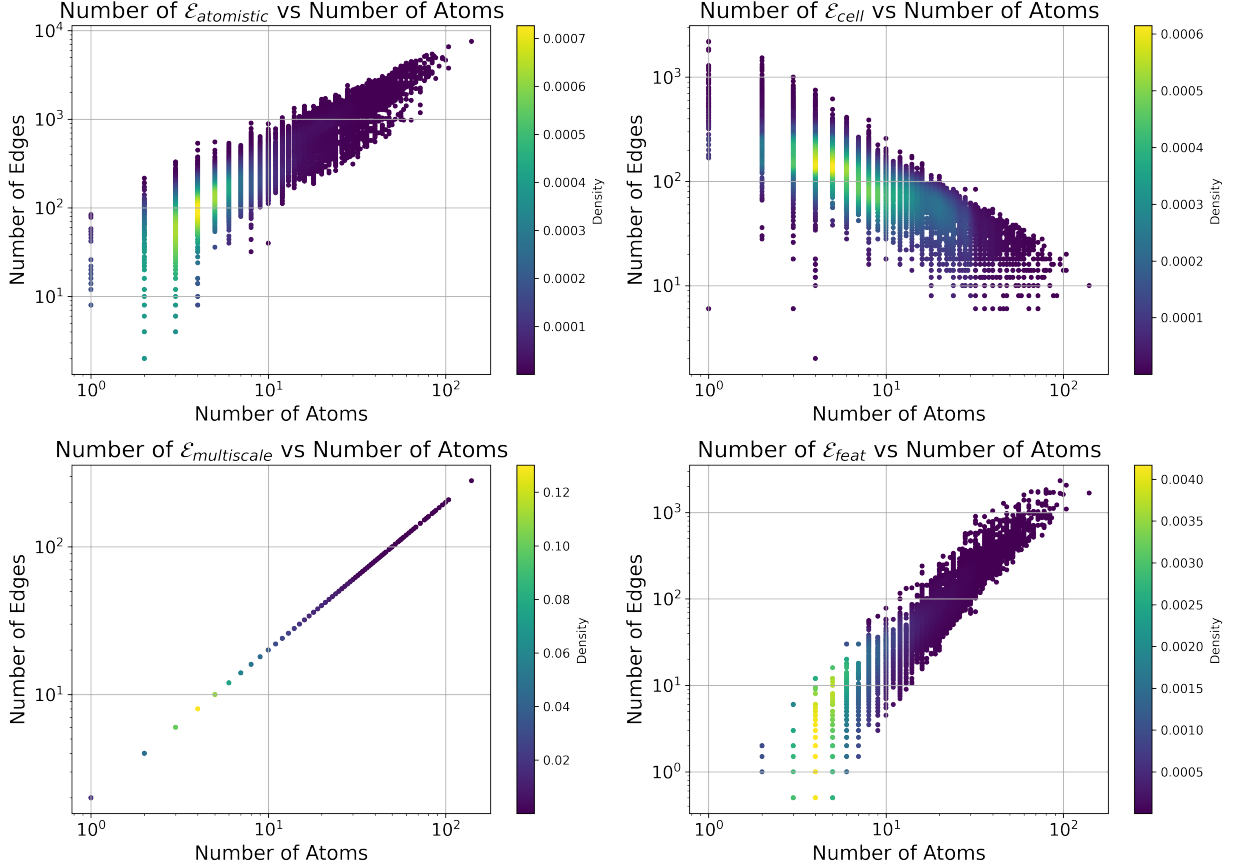

Figure 3: Log-log scatter plots of atomistic edges  $\mathcal{E}_{\text{atomistic}}$  (upper-left), cell edges  $\mathcal{E}_{\text{cell}}$  (upper-right), multiscale edges  $\mathcal{E}_{\text{multiscale}}$  (lower-left), and feature-space edges  $\mathcal{E}_{\text{feat}}$  (lower-right) versus number of atoms  $N$ .

Figure 4 focuses on the feature-space expert across the four message-passing layers. The nearly identical edge counts in layers 0–3 show that each depth learns a stable similarity threshold. A slight downward trend at large  $N$  indicates that, as embeddings become more discriminative, fewer atom pairs exceed the cutoff.

Based on the empirical data from the JARVIS formation-energy dataset, we can approxi-

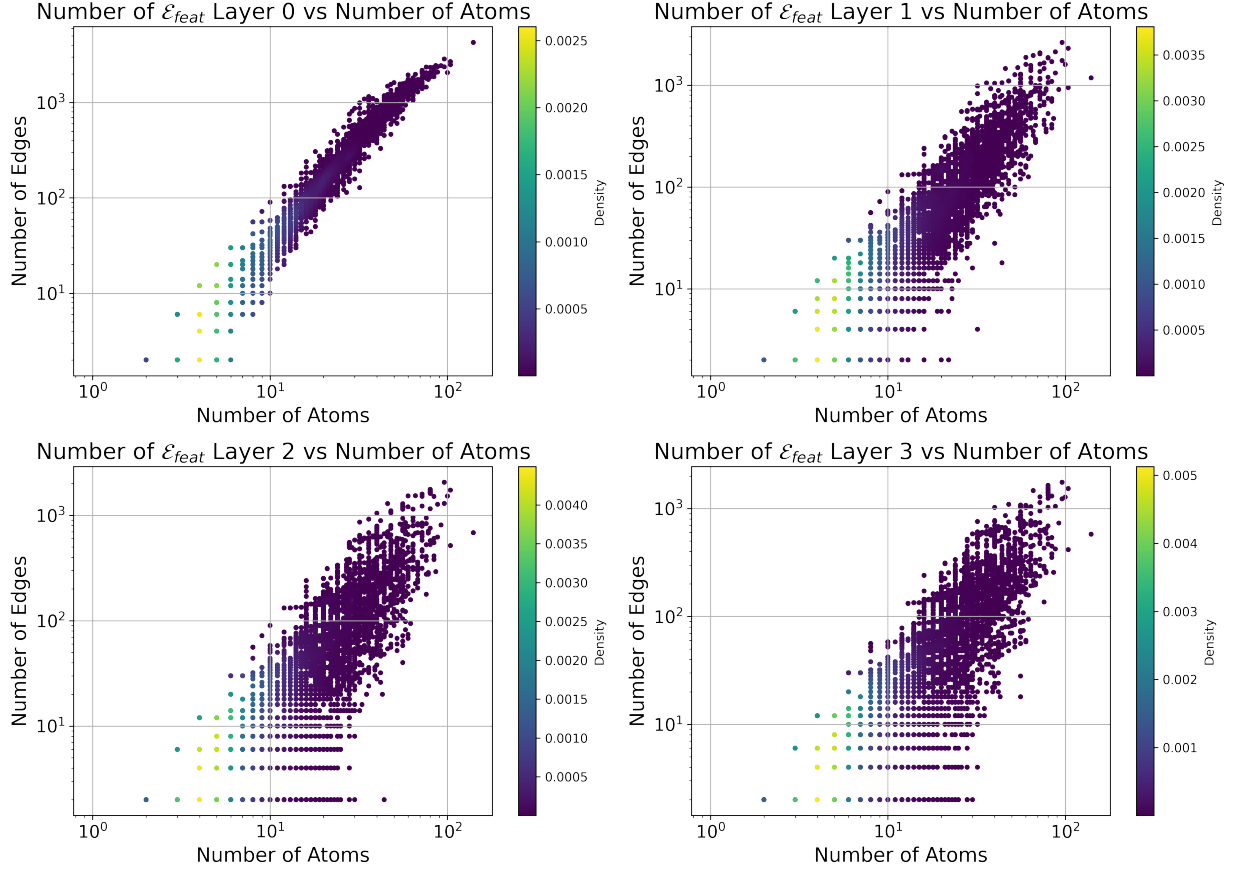

Figure 4: Log-log scatter plots of  $\mathcal{E}_{\text{feat}}$  for each model layer versus number of atoms  $N$ .

mate by a linear regression that:

$$\mathcal{E}_{\text{atomistic}} = 43.38N, \quad \mathcal{E}_{\text{cell}} = -6.5N, \quad \mathcal{E}_{\text{feat}} = 9.15, \quad \mathcal{E}_{\text{multiscale}} = 2N.$$

Consequently,

$$\mathcal{E}_{\text{total}} = (43.38 - 6.5 + 9.15 + 2) N \approx 48 N, \quad (19)$$

demonstrating overall linear scaling  $\mathcal{O}(48N)$ .

To benchmark against existing approaches, we approximate typical neighbour counts of 43 since it is the average of the neighbours in the Jarvis dataset for 5 for radius graphs and  $k = 25$  for k-NN graphs since it is the default value for state-of-the-art methods. For the case of iComformer, they perform k-NN to create the neighbourhood, and then three messages,

one per dimension, are performed to encode the edge. Table 1 summarises the per-atom complexity and parameter counts of several state-of-the-art methods.

Table 1: Comparison of methods in terms of per-atom message-passing complexity and number of parameters. Best in **bold** and second-best underlined.

| Method     | Complexity                  | Num. Params. |
|------------|-----------------------------|--------------|
| Matformer  | $\mathcal{O}(31N)$          | <u>2.9M</u>  |
| ALIGNN     | $\mathcal{O}(625N)$         | 4.0M         |
| PotNet     | $\mathcal{O}(N^2)$          | 1.76M        |
| eComFormer | $\mathcal{O}(\mathbf{25N})$ | 12.4M        |
| iComFormer | $\mathcal{O}(75N)$          | 5.0M         |
| CartNet    | $\mathcal{O}(43N)$          | <b>2.5M</b>  |
| PRISM      | $\mathcal{O}(48N)$          | 9M           |

PRISM’s  $\mathcal{O}(48N)$  scaling places similar to the radius-graph models (e.g. CartNet  $\mathcal{O}(43N)$ ). The number of parameters (9M) lies between iComformer (5M) and eComformer (12.4M). The enhanced global and feature-space interactions justify the moderate constant factor, yielding improved accuracy while maintaining practical efficiency.

## Datasets Description

**JARVIS 3D DFT Dataset.** The JARVIS 3D DFT Dataset (version 2021.8.18)<sup>4</sup> comprises approximately 55 000 bulk crystal structures with properties computed via density functional theory (DFT) under the OptB88-vdW<sup>5</sup> functional for both geometry optimization and subsequent property evaluation. It includes:

- Formation energy (meV/atom), indicating thermodynamic stability relative to elemental reference states.
- Band gap (OPT, eV), the Kohn–Sham gap computed within the OptB88-vdW approximation.
- Total energy (eV), the ground-state energy of the optimized cell.

- Band gap (MBJ, eV), a subset of  $\sim 18\,000$  structures recomputed with the Tran–Blaha modified Becke–Johnson potential for improved gap accuracy.<sup>6</sup>
- Energy above hull (Ehull, meV/atom), measuring metastability against phase decomposition.

**Materials Project Dataset.** The Materials Project Dataset (release 2018.6.1)<sup>7</sup> contains roughly 69 000 inorganic crystals optimized at the PBE-D3(BJ)<sup>8,9</sup> level of theory. Reported properties include formation energy, band gap, bulk modulus (log GPa), and shear modulus (log GPa). Note that bulk and shear moduli are available for only  $\sim 5\,500$  structures, posing a moderate low-data challenge.

**MatBench.** MatBench<sup>10</sup> is a community-driven suite of crystal-property prediction tasks spanning diverse data regimes. We adopt two representative tasks:

- **e\_form**: formation-energy prediction on 132 752 crystals.
- **jdft2d**: elastic-property prediction on 636 two-dimensional crystal structures.

We follow the official MatBench evaluation protocol, reporting mean absolute error (MAE) and root-mean-square error (RMSE) averaged over five random seeds, with standard deviations to quantify uncertainty.

These datasets together span over two orders of magnitude in size and include both large-scale (JARVIS, e\_form) and small-scale (MBJ band gaps, jdft2d) tasks, enabling a thorough assessment of PRISM’s accuracy and scalability across material-property prediction regimes.

## Training Details

Experiments were conducted on a single NVIDIA RTX 3090 GPU (24 GB memory) and a host system with two AMD EPYC 7313 16-core CPUs. All implementations use PyTorch

v2.4.0<sup>11</sup> and PyTorch Geometric v2.6.1.<sup>12</sup>

Unless otherwise specified, models consist of four PRISM layers with feature dimension  $d = 256$  and are trained with a batch size of 64. We apply SO(3) rotational data augmentation as in CartNet<sup>2</sup> and optimize using the  $L_1$  loss.

In most experiments, we use the AdamW-ScheduleFree optimizer.<sup>13</sup> For some other properties we instead employ the Adam optimizer<sup>14</sup> with a OneCycle learning rate scheduler (pct\_start=0.01).<sup>15</sup> Other hyperparameters—including the learning rate, momentum coefficients  $(\beta_1, \beta_2)$ , and cutoff radii  $(r_c, R_c, r_f)$ —are tuned per task.

## JARVIS Dataset

Table 2 lists the hyperparameters used for the JARVIS benchmark.

Table 2: Hyperparameters for the JARVIS dataset.

| Property          | Optimizer          | LR                 | $(\beta_1, \beta_2)$ | Scheduler | Weight Decay | Epochs | SO(3) Aug. | $r_c$ | $R_c$ | $r_f$ |
|-------------------|--------------------|--------------------|----------------------|-----------|--------------|--------|------------|-------|-------|-------|
| Formation Energy  | AdamW-ScheduleFree | $1 \times 10^{-3}$ | (0.9, 0.999)         | None      | 0            | 500    | Yes        | 5 Å   | 15 Å  | 1     |
| Band Gap (OPT)    | AdamW-ScheduleFree | $1 \times 10^{-3}$ | (0.9, 0.999)         | None      | 0            | 500    | Yes        | 5 Å   | 15 Å  | 1     |
| Total Energy      | Adam               | $1 \times 10^{-3}$ | (0.9, 0.999)         | OneCycle  | 0            | 500    | Yes        | 5 Å   | 15 Å  | 1     |
| Band Gap (MBJ)    | Adam               | $1 \times 10^{-3}$ | (0.9, 0.999)         | OneCycle  | 0            | 500    | Yes        | 5 Å   | 15 Å  | 1     |
| $E_{\text{hull}}$ | Adam               | $1 \times 10^{-3}$ | (0.9, 0.999)         | OneCycle  | 0            | 500    | Yes        | 5 Å   | 30 Å  | 1     |

## Materials Project Dataset

Table 3 presents the hyperparameters for the Materials Project dataset.

Table 3: Hyperparameters for the Materials Project dataset.

| Property         | Optimizer          | LR                 | $(\beta_1, \beta_2)$ | Scheduler | Weight Decay       | Epochs | SO(3) Aug. | $r_c$ | $R_c$ | $r_f$ |
|------------------|--------------------|--------------------|----------------------|-----------|--------------------|--------|------------|-------|-------|-------|
| Formation Energy | AdamW-ScheduleFree | $1 \times 10^{-3}$ | (0.9, 0.999)         | None      | $1 \times 10^{-6}$ | 500    | Yes        | 5 Å   | 15 Å  | 1     |
| Band Gap         | AdamW-ScheduleFree | $1 \times 10^{-3}$ | (0.9, 0.999)         | None      | $1 \times 10^{-6}$ | 500    | Yes        | 5 Å   | 15 Å  | 1     |
| Shear Moduli     | Adam               | $1 \times 10^{-3}$ | (0.9, 0.999)         | OneCycle  | 0                  | 1000   | Yes        | 5 Å   | 15 Å  | 1     |
| Bulk Moduli      | Adam               | $1 \times 10^{-3}$ | (0.9, 0.999)         | OneCycle  | $1 \times 10^{-6}$ | 500    | No         | 5 Å   | 30 Å  | 1     |

# Matbench Dataset

Table 4 details the hyperparameters for the Matbench tasks. For the `jdfft2d` task, we insert a dropout layer (rate 0.5) between the final atomic embeddings and the prediction head.

Table 4: Hyperparameters for the Matbench dataset.

| Property             | Optimizer          | LR                 | $(\beta_1, \beta_2)$ | Scheduler | Weight Decay       | Epochs | SO(3) Aug. | $r_c$ | $R_c$ | $r_f$ |
|----------------------|--------------------|--------------------|----------------------|-----------|--------------------|--------|------------|-------|-------|-------|
| e_form               | AdamW-ScheduleFree | $1 \times 10^{-3}$ | (0.95, 0.999)        | None      | 0                  | 500    | Yes        | 5 Å   | 15 Å  | 1     |
| jdf <sub>ft</sub> 2d | AdamW-ScheduleFree | $1 \times 10^{-3}$ | (0.95, 0.999)        | None      | $1 \times 10^{-6}$ | 5000   | Yes        | 5 Å   | 15 Å  | 1     |

# References

- (1) Yan, K.; Fu, C.; Qian, X.; Qian, X.; Ji, S. Complete and Efficient Graph Transformers for Crystal Material Property Prediction. International Conference on Learning Representations. 2024.
- (2) Solé, À.; Mosella-Montoro, A.; Cardona, J.; Gómez-Coca, S.; Aravena, D.; Ruiz, E.; Ruiz-Hidalgo, J. A Cartesian encoding graph neural network for crystal structure property prediction: application to thermal ellipsoid estimation. *Digital Discovery* **2025**, *4*, 694–710.
- (3) Elfving, S.; Uchibe, E.; Doya, K. Sigmoid-weighted linear units for neural network function approximation in reinforcement learning. *Neural Networks* **2018**, *107*, 3–11, Special issue on deep reinforcement learning.
- (4) Choudhary, K. et al. The joint automated repository for various integrated simulations (JARVIS) for data-driven materials design. *npj Computational Materials* **2020**, *6*, 173.
- (5) Klimeš, J. c. v.; Bowler, D. R.; Michaelides, A. Van der Waals density functionals applied to solids. *Phys. Rev. B* **2011**, *83*, 195131.
- (6) Rai, D.; Ghimire, M.; Thapa, R. A DFT study of BeX (X= S, Se, Te) semiconductor: modified Becke Johnson (mBJ) potential. *Semiconductors* **2014**, *48*, 1411–1422.

- (7) Chen, C.; Ye, W.; Zuo, Y.; Zheng, C.; Ong, S. P. Graph Networks as a Universal Machine Learning Framework for Molecules and Crystals. *Chemistry of Materials* **2019**, *31*, 3564–3572.
- (8) Perdew, J. P.; Burke, K.; Ernzerhof, M. Generalized Gradient Approximation Made Simple. *Phys. Rev. Lett.* **1996**, *77*, 3865–3868.
- (9) Grimme, S.; Ehrlich, S.; Goerigk, L. Effect of the damping function in dispersion corrected density functional theory. *Journal of Computational Chemistry* **2011**, *32*, 1456–1465.
- (10) Dunn, A.; Wang, Q.; Ganose, A.; Dopp, D.; Jain, A. Benchmarking materials property prediction methods: the Matbench test set and Automatminer reference algorithm. *npj Computational Materials* **2020**, *6*, 138.
- (11) Paszke, A. Pytorch: An imperative style, high-performance deep learning library. *arXiv preprint arXiv:1912.01703* **2019**,
- (12) Fey, M.; Lenssen, J. E. Fast graph representation learning with PyTorch Geometric. *arXiv preprint arXiv:1903.02428* **2019**,
- (13) Defazio, A.; Yang, X.; Khaled, A.; Mishchenko, K.; Mehta, H.; Cutkosky, A. The road less scheduled. *Advances in Neural Information Processing Systems* **2024**, *37*, 9974–10007.
- (14) Kingma, D.; Ba, J. Adam: A Method for Stochastic Optimization. International Conference on Learning Representations (ICLR). San Diego, CA, USA, 2015.
- (15) Smith, L. N.; Topin, N. Super-convergence: Very fast training of neural networks using large learning rates. Artificial intelligence and machine learning for multi-domain operations applications. 2019; pp 369–386.
